# Supplementary material for: Fractional Charges in the Su-Schrieffer-Heeger Model
Source: arXiv:2209.05981 source file (2022-06-20)
Supplement: Supplementary file 1 [file supp.pdf]

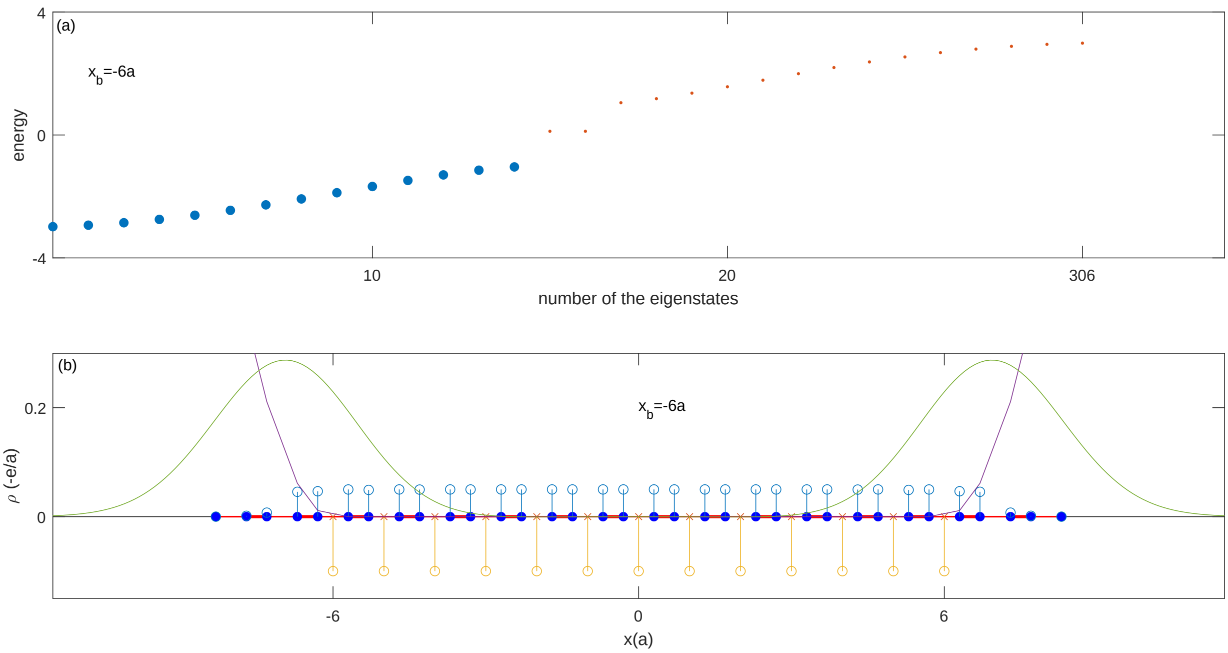


FIG. S1. (a)Eigenenergies of the SSH chain with onsite potential. The occupied states are represented by bigger dots and the edge states are empty. The onsite potential is illustrated in(b). The charge distribution and "macro" charge density are also shown in (b). Here $\lambda = -2$, $\gamma = -1$ and $D = a$.

## I. EFFECT OF DIFFERENT BOUNDARY CONDITIONS AND RANDOM DISORDERS ON THE FRACTIONAL CHARGE AT THE BOUNDARY

To show that the fractional charge does not depend on the choice of boundary we use a more complicated model for the boundary. We assume the sites are located at $x_i(n)$, where $i = A$ and $i = B$ are shown in the main text. $x_A(n) = (n + 0.3)a$, $x_B(n) = (n - 0.3)a$ and $n = -8, -7, ...8$. We add an onsite potential $V = (x_i - x_b)^2$ when $x_i <= x_b$ at the left end of the chain and an onsite potential to the right end to preserve the inversion symmetry of the system. When $x_b$ continuously increases from $-6a$ to $-5a$ the boundary with be translated by one lattice constant $a$. We show in Fig.S1-S4 the fractional charge always presents at the edge regardless the existence of the edge states or not.

To study the effect of random disorders on the fractional charge we first add random hopping $t_r$ to $\lambda$ and $\gamma$, where $t_r$ uniformly distributed from $-t_0$ to $t_0$. We this type of disorders have little effect on the rational charge. We use $t_0$ as large as $|\gamma|$ and the fractional charge is still very close to $e/2$ as shown in Fig.S5.

We also add random onsite potentials $V_r$ to the system, where $V_r$ uniformly distributed from $-V_0$ to $V_0$. In this case there are greater charge density fluctuations in the bulk. It is impossible to separate the charge at the boundary and the bulk charge fluctuations. Thus the charge at boundary will deviate from $e/2$ significantly as shown in Fig.S6. However, the ensemble average approaches $e/2$ when the sample size is large enough. We run the simulations for 10000 times and the average $Q_l$ and $Q_r$ are very close to $e/2$ as shown in Fig.S7.

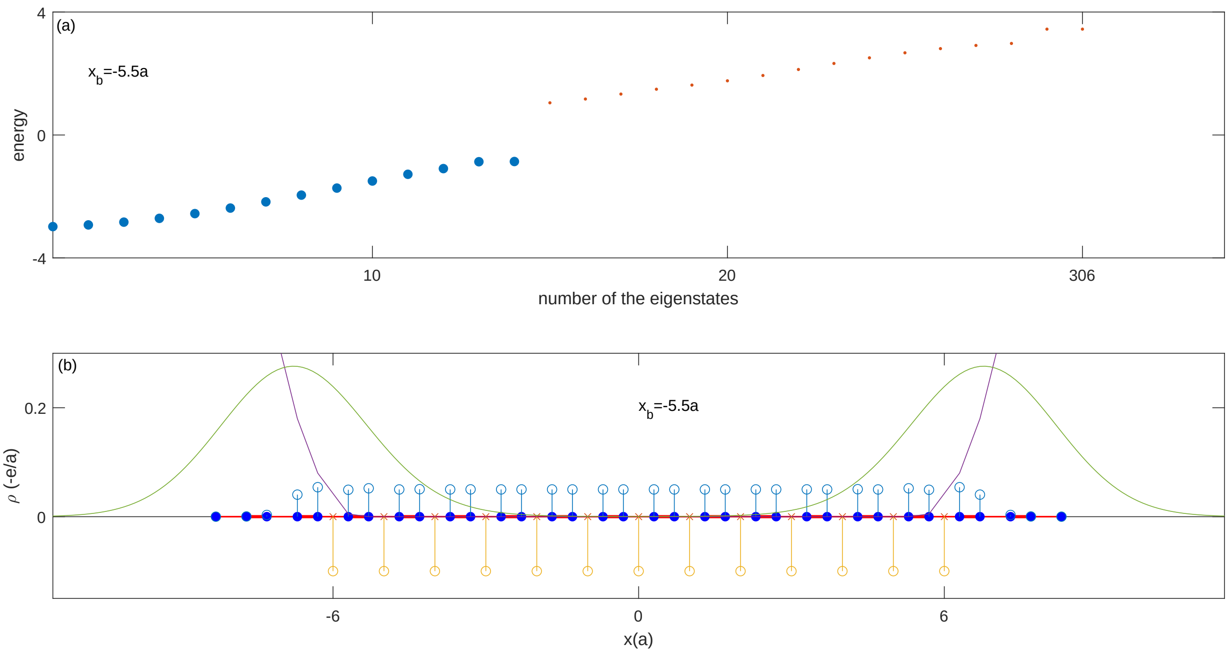


FIG. S2. (a)Eigenenergies of the SSH chain with onsite potential. There is no edge states in the bulk gap. The onsite potential is illustrated in(b). The charge distribution and “macro” charge density are also shown in (b). Here $\lambda = -2$, $\gamma = -1$ and $D = a$.

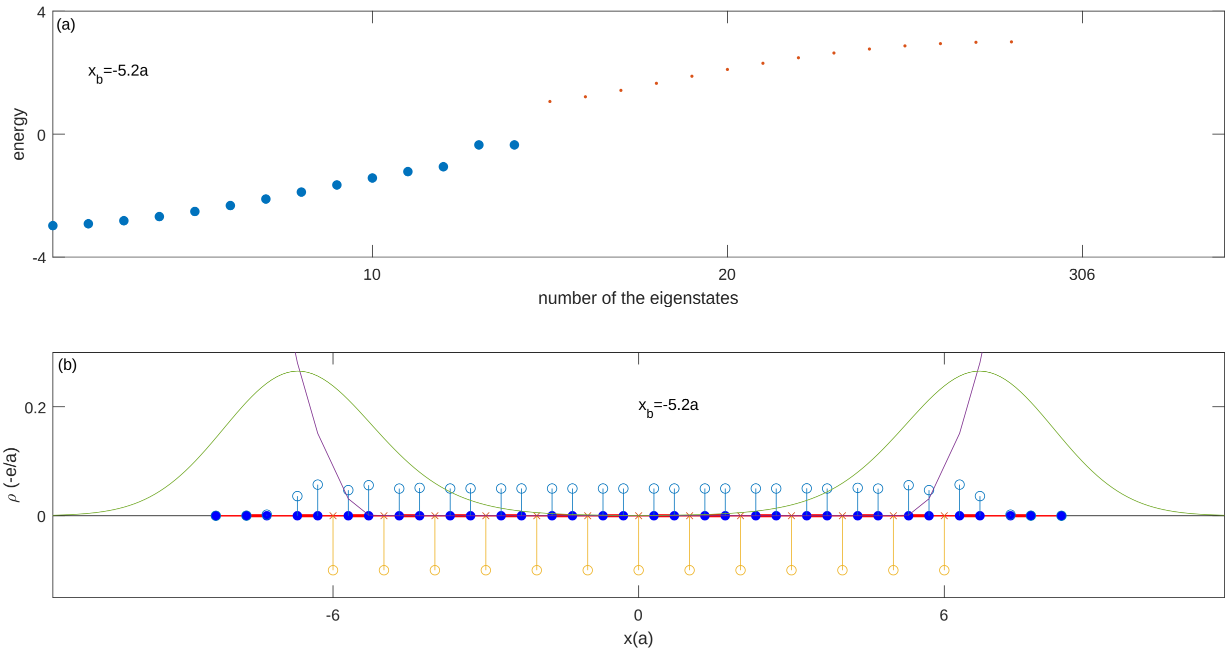


FIG. S3. (a)Eigenenergies of the SSH chain with onsite potential. The occupied states are represented by bigger dots and the edge states are full. The onsite potential is illustrated in(b). The charge distribution and “macro” charge density are also shown in (b). Here $\lambda = -2$, $\gamma = -1$ and $D = a$.

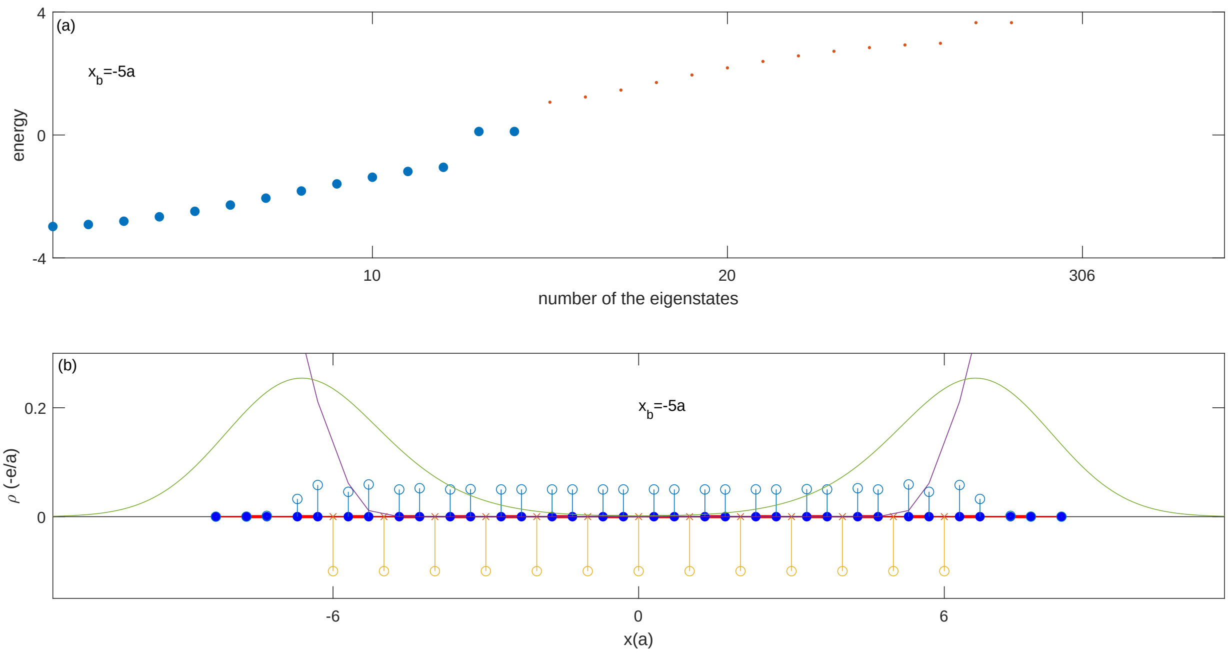


FIG. S4. (a)Eigenenergies of the SSH chain with onsite potential. The occupied states are represented by bigger dots and the edge states are full. The onsite potential is illustrated in(b). The charge distribution and "macro" charge density are also shown in (b). Here $\lambda = -2$, $\gamma = -1$ and $D = a$.

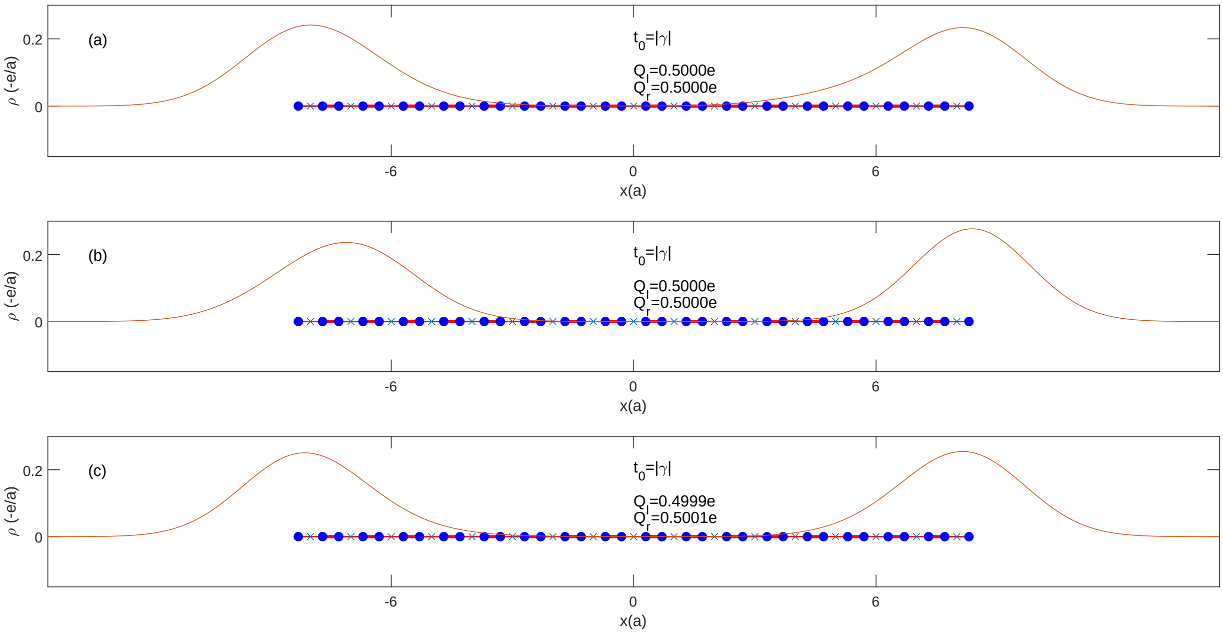


FIG. S5. (a)-(c)Charge densities of the SSH chain with random $t_r$. Values of charges at the left and right boundaries are denoted by $Q_l$ and $Q_r$. (a)-(c) correspond to three different simulations.

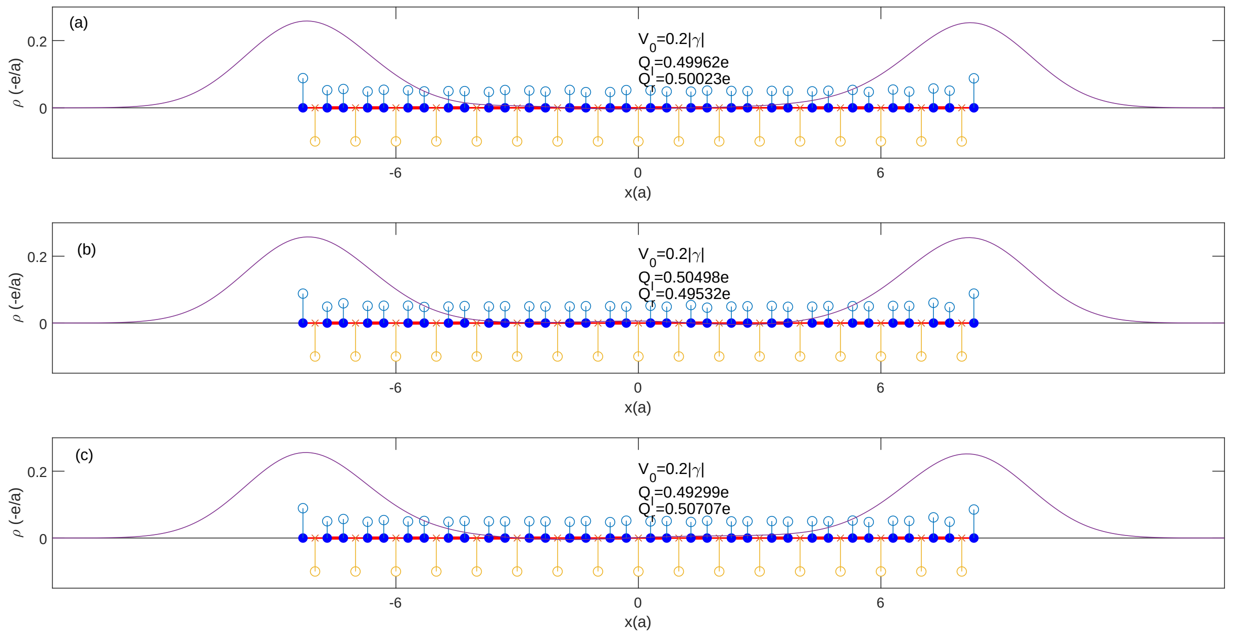


FIG. S6. (a)-(c)Charge densities of the SSH chain with random onesite potentials. Values of charges at the left and right boundaries are denoted by $Q_l$ and $Q_r$. (a)-(c) correspond to three different simulations.

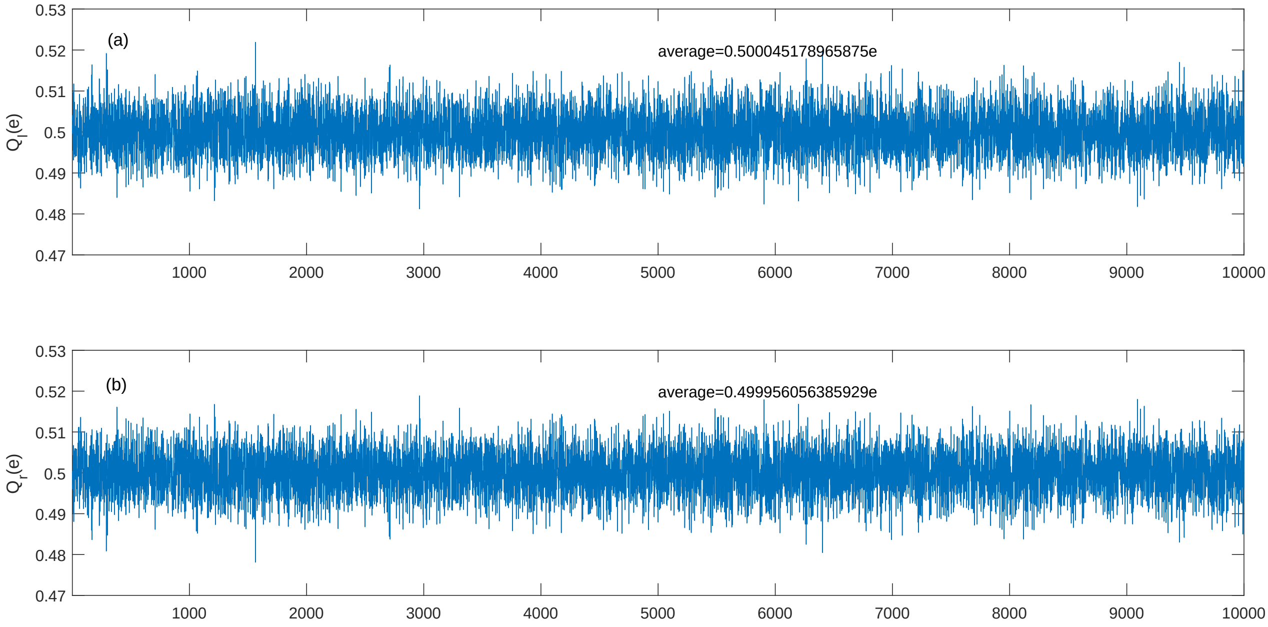


FIG. S7. (a)and(b)Charges at the boundaries with 10000 times of simulations. Here $V_0 = 0.2|\gamma|$.
